# Supplementary material for: VIP: Video Inpainting Pipeline for Real World Human Removal
Source: arXiv:2504.03041 source file (2025-04-03)
Supplement: Supplementary file 1 [file supp.tex]

\begin{figure}[htbp]
\centering
\footnotesize
\includegraphics[width=1\linewidth]{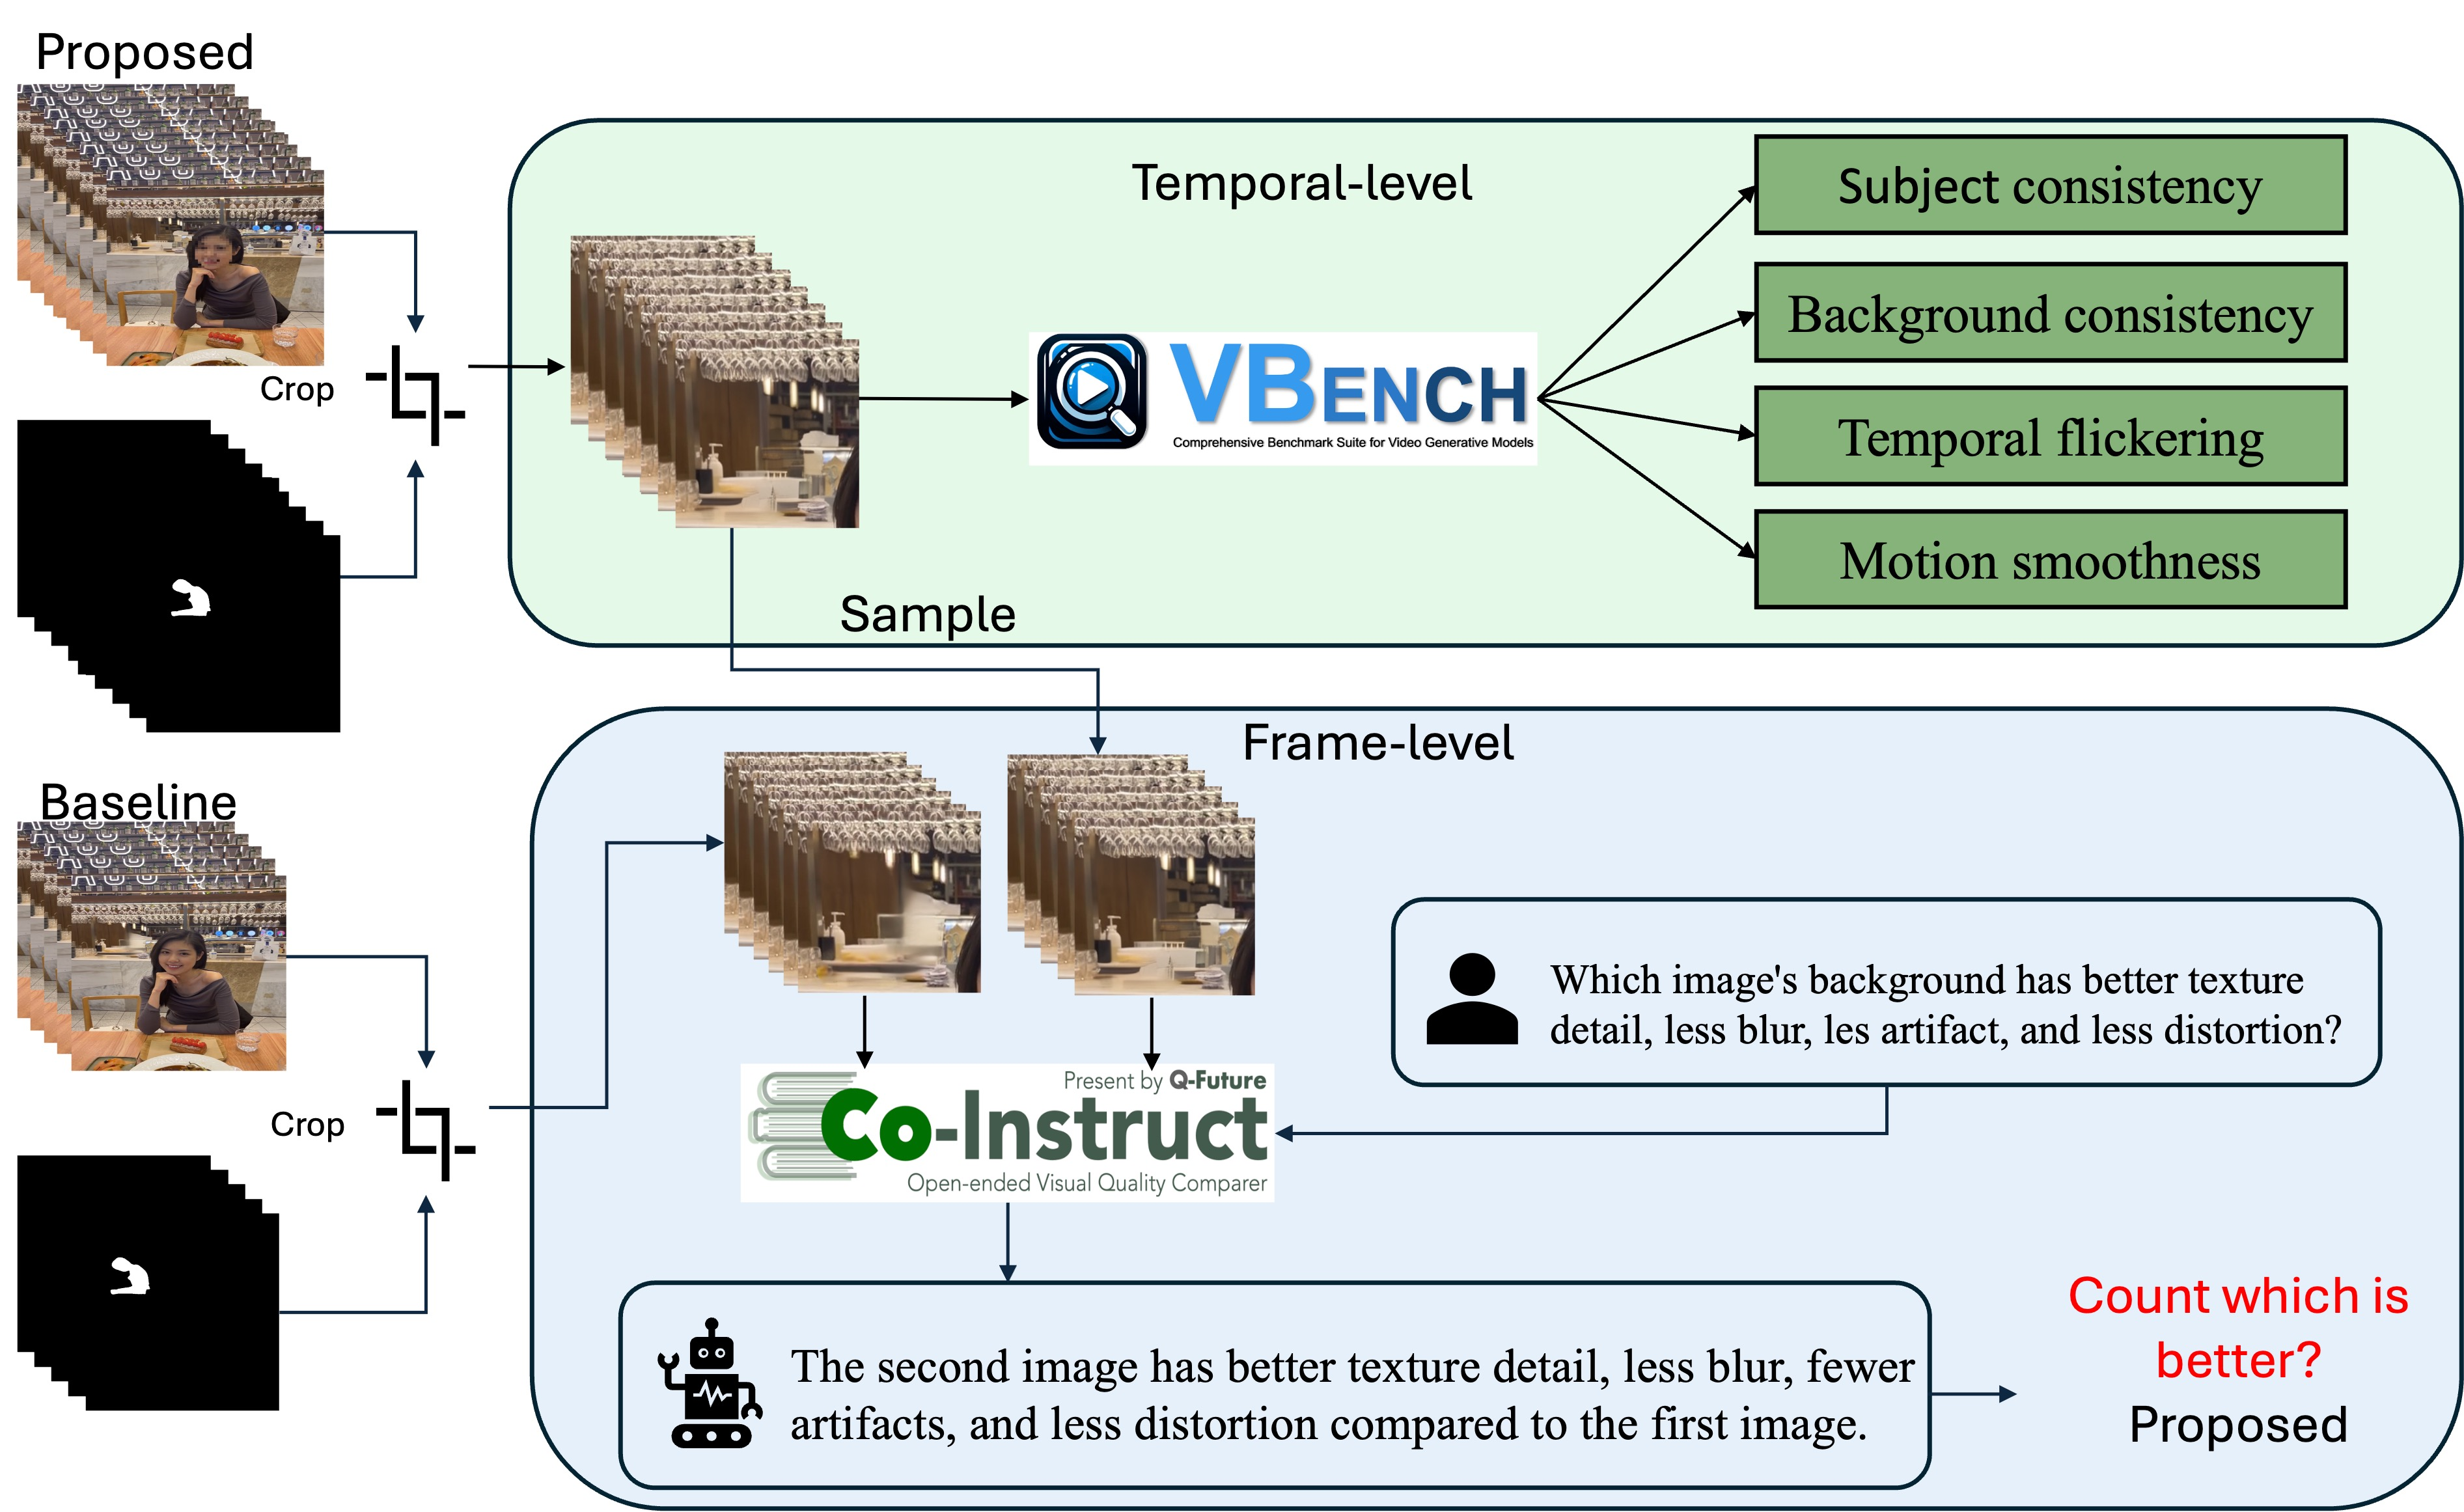}

\caption{ \hm{needs update} }
\label{fig:evaluation}	 
\end{figure}

1.We use WebVid~\cite{Bain21} dataset as the beginning training dataset in a size of $256 \times 256$, with the learning rate $5e^{-5}$ and batch size 1024 for 200K steps. 2. We do image and video joint training in the second stage, we use ACAV~\cite{lee2021acav100m} dataset and LAION~\cite{schuhmann2022laion} with the 512 batch size for 400K steps, the text prompt is also only kept to "inpainting". We combine 24 individual images to a video sequence and send it to the video diffusion model. The images and video frame are in a size of $24 \times 512 \times 512$ and the learning rate $1e^{-5}$. 3. At the final stage, for 50\% of the training samples clip, we randomly selected one frame and didn't apply the mask on it's frame and mask input. we train the model on our custom self-collected dataset in size of $640 \times 640$ for a batch size of 192 and the learning rate $1e^{-5}$ for 400K steps.

 Our evaluation protocol samples 5 frames per video and focuses on the inpainted regions to ensure targeted assessment of the removal areas. The final performance is the win rate of each method in pairwise comparisons.
